# Supplementary material for: Learning to Evaluate Before Improving: Automatic Rubric Induction for Automatic Research Agents
Source: arXiv:2608.31076 source file (2026-08-31)
Supplement: Supplementary file 1 [file appendix.tex]

\documentclass[letterpaper]{article} % DO NOT CHANGE THIS
\usepackage[submission]{aaai2027}  % DO NOT CHANGE THIS
% The serif, sans-serif, and monospaced fonts are loaded automatically by
% aaai2027.sty (newtxtext, helvet, courier). DO NOT add \usepackage{times},
% \usepackage{helvet}, \usepackage{courier}, or any other font package.
\usepackage[hyphens]{url}  % DO NOT CHANGE THIS
\usepackage{graphicx} % DO NOT CHANGE THIS
\urlstyle{rm} % DO NOT CHANGE THIS
\def\UrlFont{\rm}  % DO NOT CHANGE THIS
\usepackage{natbib}  % DO NOT CHANGE THIS AND DO NOT ADD ANY OPTIONS TO IT
\usepackage{caption} % DO NOT CHANGE THIS AND DO NOT ADD ANY OPTIONS TO IT
\frenchspacing  % DO NOT CHANGE THIS
%
% These are recommended to typeset algorithms but not required. See the subsubsection on algorithms. Remove them if you don't have algorithms in your paper.
\usepackage{algorithm}
\usepackage{algorithmic}
\usepackage{amsmath}
\usepackage{amssymb}
\usepackage{tabularx}
\usepackage{array}


%prompt
\usepackage[most]{tcolorbox}
\usepackage{listings}
\usepackage{xcolor}

\definecolor{PromptFrame}{HTML}{6F927D}
\definecolor{PromptBackground}{HTML}{EEF7F1}

\newtcblisting{PromptBox}[1]{
  enhanced,
  breakable,
  listing only,
  title={#1},
  colback=PromptBackground,
  colframe=PromptFrame,
  colbacktitle=PromptFrame,
  coltitle=white,
  fonttitle=\bfseries\small,
  boxrule=0.7pt,
  arc=2pt,
  left=2mm,
  right=2mm,
  top=1.5mm,
  bottom=1.5mm,
  before skip=8pt,
  after skip=10pt,
  listing options={
    basicstyle=\rmfamily\footnotesize,
    numbers=none,
    numberstyle=\scriptsize,
    breaklines=true,
    breakatwhitespace=true,
    breakautoindent=false,
    breakindent=0pt,
    columns=fullflexible,
    keepspaces=true,
    showspaces=false,
    showstringspaces=false,
    showtabs=false,
    tabsize=2,
    xleftmargin=0pt,
    frame=none,
    aboveskip=0pt,
    belowskip=0pt
  }
}
%
% These are recommended to typeset listings but not required. See the subsubsection on listing. Remove this block if you don't have listings in your paper.
\usepackage{newfloat}
\usepackage{listings}
\DeclareCaptionStyle{ruled}{labelfont=normalfont,labelsep=colon,strut=off} % DO NOT CHANGE THIS
\lstset{%
	basicstyle={\footnotesize\ttfamily},% footnotesize acceptable for monospace
	numbers=left,numberstyle=\footnotesize,xleftmargin=2em,% show line numbers, remove this entire line if you don't want the numbers.
	aboveskip=0pt,belowskip=0pt,%
	showstringspaces=false,tabsize=2,breaklines=true}
\floatstyle{ruled}
\newfloat{listing}{tb}{lst}{}
\floatname{listing}{Listing}

%
% Recommended for better-looking tables
\usepackage{booktabs}
\usepackage{graphicx}
\usepackage{subcaption}

\captionsetup[subfigure]{
    font=small,
    labelfont=bf,
    justification=centering,
    singlelinecheck=true
}
%
% Keep the \pdfinfo as shown here. There's no need
% for you to add the /Title and /Author tags.
\pdfinfo{
/TemplateVersion (2027.1)
}
\usepackage{booktabs}
\usepackage{multirow}
\usepackage{graphicx}
\usepackage[table,dvipsnames]{xcolor}
\usepackage{makecell}
% ============================================================
% Required packages
% ============================================================
% \usepackage{booktabs}
% \usepackage[table,dvipsnames]{xcolor}
% \usepackage{graphicx}
% \usepackage{makecell}

% ============================================================
% Color definitions
% ============================================================
\definecolor{GainGreen}{HTML}{169B45}
\definecolor{LossRed}{HTML}{D64545}
\definecolor{PanelBlue}{HTML}{EAF2FF}
\definecolor{HeaderBlue}{HTML}{F5F8FD}
\definecolor{OursBlue}{HTML}{F8FAFF}
\definecolor{NoteGray}{HTML}{667085}

% ============================================================
% Gain / loss annotations
% ============================================================
\newcommand{\scoregain}[1]{%
  \hspace{0.12em}%
  {\scriptsize\bfseries\textcolor{GainGreen}{$\uparrow$\,#1}}%
}

\newcommand{\scoreloss}[1]{%
  \hspace{0.12em}%
  {\scriptsize\bfseries\textcolor{LossRed}{$\downarrow$\,#1}}%
}

\usepackage{pifont}

\newcommand{\cmark}{\ding{51}}
\newcommand{\xmark}{\ding{55}}

% ============================================================
% Model / harness icons
% ============================================================

\newcommand{\RcbIcon}[1]{%
  \IfFileExists{Figures/logos/#1.png}{%
    \raisebox{-0.13em}{%
      \includegraphics[
        draft=false,
        height=0.90em,
        keepaspectratio
      ]{Figures/logos/#1.png}%
    }%
  }{%
    \PackageWarning{MainTable}{Icon Figures/logos/#1.png not found}%
    \makebox[0.90em][c]{\scriptsize ?}%
  }%
  \hspace{0.20em}%
}

% Backbone LLM icons
\newcommand{\OpenAIIcon}{\RcbIcon{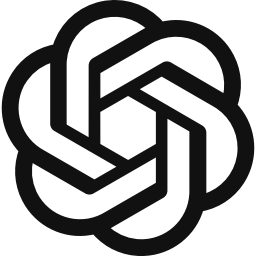}}
\newcommand{\GlmIcon}{\RcbIcon{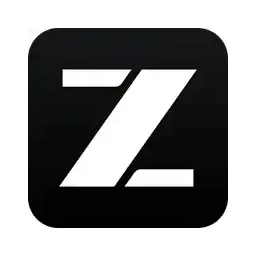}}
\newcommand{\MiniMaxIcon}{\RcbIcon{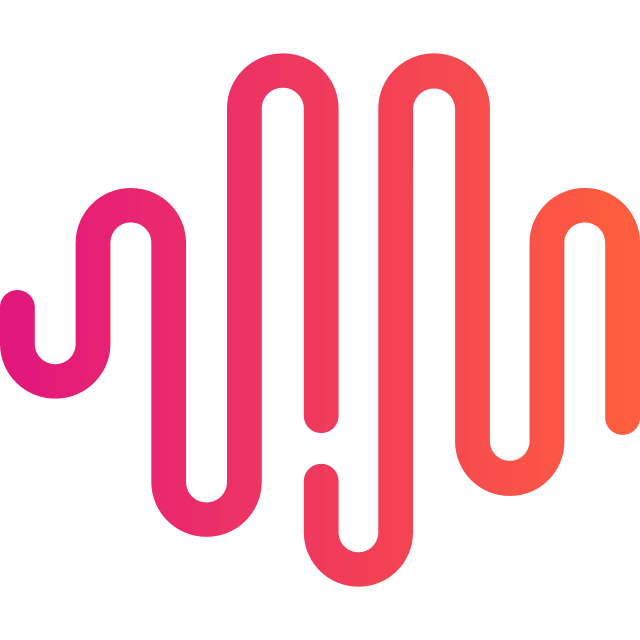}}
\newcommand{\DeepSeekIcon}{\RcbIcon{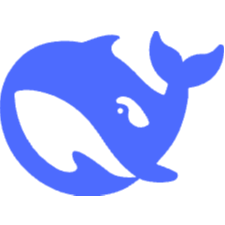}}

% Agent harness icons
\newcommand{\CodexIcon}{\RcbIcon{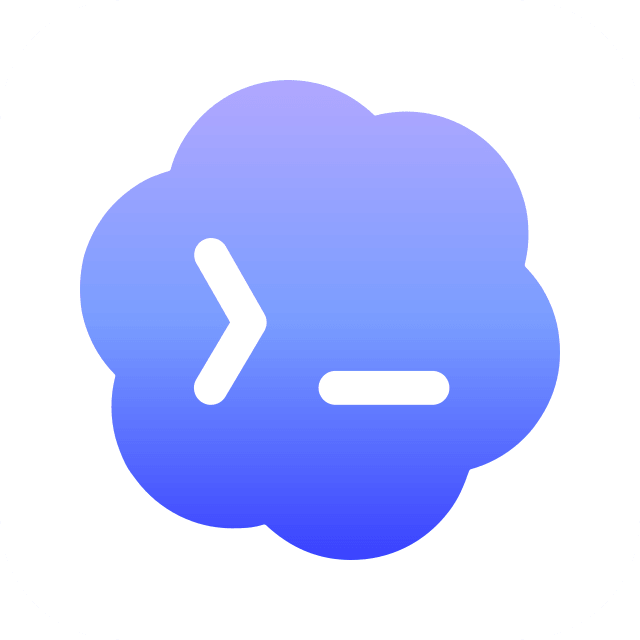}}
\newcommand{\ClaudeIcon}{\RcbIcon{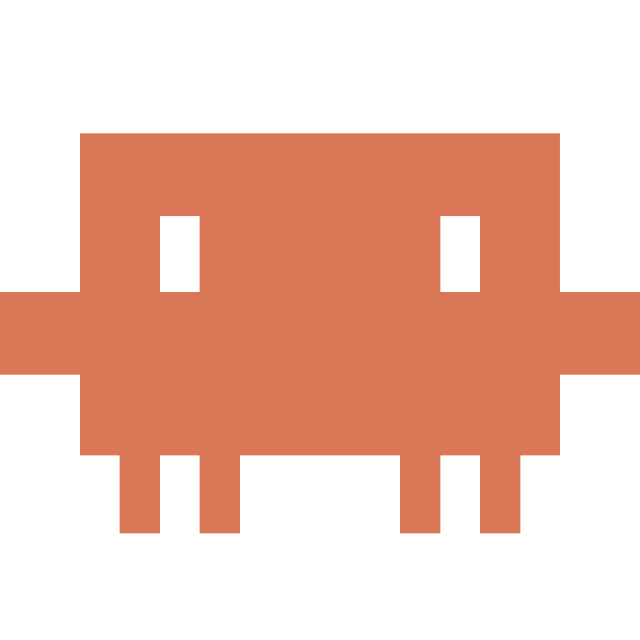}}
\newcommand{\OpenClawIcon}{\RcbIcon{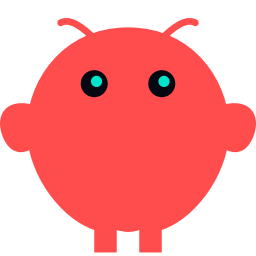}}
\newcommand{\OpenScienceIcon}{\RcbIcon{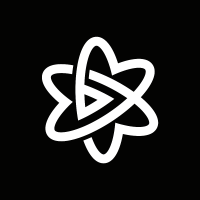}}

% Place the model/harness name in the second row and merge upward.
% \cellcolor{white} prevents the blue ours-row background from
% entering the merged model/harness cell.
\newcommand{\ModelCell}[2]{%
  \cellcolor{white}%
  \multirow{-2}{*}[-0.10ex]{%
    \begingroup
    \setlength{\fboxsep}{0pt}%
    \colorbox{white}{\strut #1#2}%
    \endgroup
  }%
}

% ============================================================
% Overall-column highlighting
% ============================================================
\definecolor{OverallHeaderBlue}{HTML}{DCE8F5}
\definecolor{OverallVanillaBlue}{HTML}{F2F6FA}
\definecolor{OverallOursBlue}{HTML}{E2EDF8}

\newcommand{\OverallHeader}{%
  \cellcolor{OverallHeaderBlue}\textbf{Overall}%
}

\newcommand{\OverallVanilla}[1]{%
  \cellcolor{OverallVanillaBlue}#1%
}

\newcommand{\OverallOurs}[2]{%
  \cellcolor{OverallOursBlue}%
  \textbf{#1}\scoregain{#2}%
}
% Required:
% \usepackage{xcolor}

% \newcommand{\scoreorig}[1]{%
%   \makebox[2.35em][r]{#1}%
%   \makebox[3.10em][l]{}%
% }

% \newcommand{\scoregaincell}[2]{%
%   \makebox[2.35em][r]{\textbf{#1}}%
%   \makebox[3.10em][l]{%
%     \raisebox{-0.45ex}{\scriptsize\textcolor{green!50!black}{\ensuremath{(+#2)}}}%
%   }%
% }

% \newcommand{\scorelosscell}[2]{%
%   \makebox[2.35em][r]{\textbf{#1}}%
%   \makebox[3.10em][l]{%
%     \raisebox{-0.45ex}{\scriptsize\textcolor{red!70!black}{\ensuremath{(-#2)}}}%
%   }%
% }
\newcommand{\our}{AutoSciRub}




% DISALLOWED PACKAGES
% \usepackage{authblk} -- This package is specifically forbidden
% \usepackage{balance} -- This package is specifically forbidden
% \usepackage{CJK} -- This package is specifically forbidden
% \usepackage{float} -- This package is specifically forbidden
% \usepackage{flushend} -- This package is specifically forbidden
% \usepackage{fullpage} -- This package is specifically forbidden
% \usepackage{geometry} -- This package is specifically forbidden
% \usepackage{hyperref} -- This package is specifically forbidden
% \usepackage{navigator} -- This package is specifically forbidden
% (or any other package that embeds links such as navigator or hyperref)
% \usepackage{indentfirst} -- This package is specifically forbidden
% \usepackage{layout} -- This package is specifically forbidden
% \usepackage{multicol} -- This package is specifically forbidden
% \usepackage{nameref} -- This package is specifically forbidden
% \usepackage{savetrees} -- This package is specifically forbidden
% \usepackage{setspace} -- This package is specifically forbidden
% \usepackage{stfloats} -- This package is specifically forbidden
% \usepackage{tabu} -- This package is specifically forbidden
% \usepackage{titlesec} -- This package is specifically forbidden
% \usepackage{tocbibind} -- This package is specifically forbidden
% \usepackage{ulem} -- This package is specifically forbidden
% \usepackage{wrapfig} -- This package is specifically forbidden
% DISALLOWED COMMANDS
% \nocopyright -- Your paper will not be published if you use this command
% \addtolength -- This command may not be used
% \balance -- This command may not be used
% \baselinestretch -- Your paper will not be published if you use this command
% \clearpage -- No page breaks of any kind may be used for the final version of your paper
% \columnsep -- This command may not be used
% \newpage -- No page breaks of any kind may be used for the final version of your paper
% \pagebreak -- No page breaks of any kind may be used for the final version of your paper
% \pagestyle -- This command may not be used
% \tiny -- This is not an acceptable font size.
% \vspace{- -- No negative value may be used in proximity of a caption, figure, table, section, subsection, subsubsection, or reference
% \vskip{- -- No negative value may be used to alter spacing above or below a caption, figure, table, section, subsection, subsubsection, or reference

\setcounter{secnumdepth}{2} %May be changed to 1 or 2 if section numbers are desired.

% The file aaai2027.sty is the style file for AAAI Press
% proceedings, working notes, and technical reports.
%

% Title

% Your title must be in mixed case, not sentence case.
% That means all verbs (including short verbs like be, is, using,and go),
% nouns, adverbs, adjectives should be capitalized, including both words in hyphenated terms, while
% articles, conjunctions, and prepositions are lower case unless they
% directly follow a colon or long dash
\title{Learning to Evaluate Before Improving: Automatic Rubric Induction for Automatic Research Agents}


\author{
    %Authors
    % All authors must be in the same font size and format.
    Written by AAAI Press Staff\textsuperscript{\rm 1}\thanks{With help from the AAAI Publications Committee.}\\
    AAAI Style Contributions by Peter Patel Schneider,
    Sunil Issar,\\
    J. Scott Penberthy,
    George Ferguson,
    Hans Guesgen,
    Francisco Cruz\equalcontrib\corresponding,
    Marc Pujol-Gonzalez\equalcontrib\corresponding
}
\affiliations{
    %Afiliations
    \textsuperscript{\rm 1}Association for the Advancement of Artificial Intelligence\\
    % If you have multiple authors and multiple affiliations
    % use superscripts in text and roman font to identify them.
    % For example,

    % Sunil Issar\textsuperscript{\rm 2},
    % J. Scott Penberthy\textsuperscript{\rm 3},
    % George Ferguson\textsuperscript{\rm 4}\corresponding,
    % Hans Guesgen\textsuperscript{\rm 5}
    % Note that the comma should be placed after the superscript

    1101 Pennsylvania Ave, NW Suite 300\\
    Washington, DC 20004 USA\\
    % email address must be in roman text type, not monospace or sans serif
    proceedings-questions@aaai.org
%
% See more examples next
}

%Example, Single Author, ->> remove \iffalse,\fi and place them surrounding AAAI title to use it
\iffalse
\title{My Publication Title --- Single Author}
\author {
    Author Name
}
\affiliations{
    Affiliation\\
    Affiliation Line 2\\
    name@example.com
}
\fi

\iffalse
%Example, Multiple Authors, ->> remove \iffalse,\fi and place them surrounding AAAI title to use it
\title{My Publication Title --- Multiple Authors}
\author {
    % Authors
    First Author Name\textsuperscript{\rm 1,\rm 2}\equalcontrib,
    Second Author Name\textsuperscript{\rm 2}\equalcontrib,
    Third Author Name\textsuperscript{\rm 1}\corresponding
}
\affiliations {
    % Affiliations
    \textsuperscript{\rm 1}Affiliation 1\\
    \textsuperscript{\rm 2}Affiliation 2\\
    firstAuthor@affiliation1.com, secondAuthor@affilation2.com, thirdAuthor@affiliation1.com
}
\fi



\begin{document}

\input{Sections/8_appendix}





\end{document}
